# Supplementary material for: First Sagittarius A* Event Horizon Telescope Results. III: Imaging of the Galactic Center Supermassive Black Hole
Source: arXiv:2311.09479 source file (2023-11-16)
Supplement: Supplementary file 1 [file appendix_dynamical_fullcoverage.tex]

\section{Inspection of variabilities: dynamical imaging with full observational coverage}

\begin{figure}
    \centering
    \includegraphics[width=\linewidth]{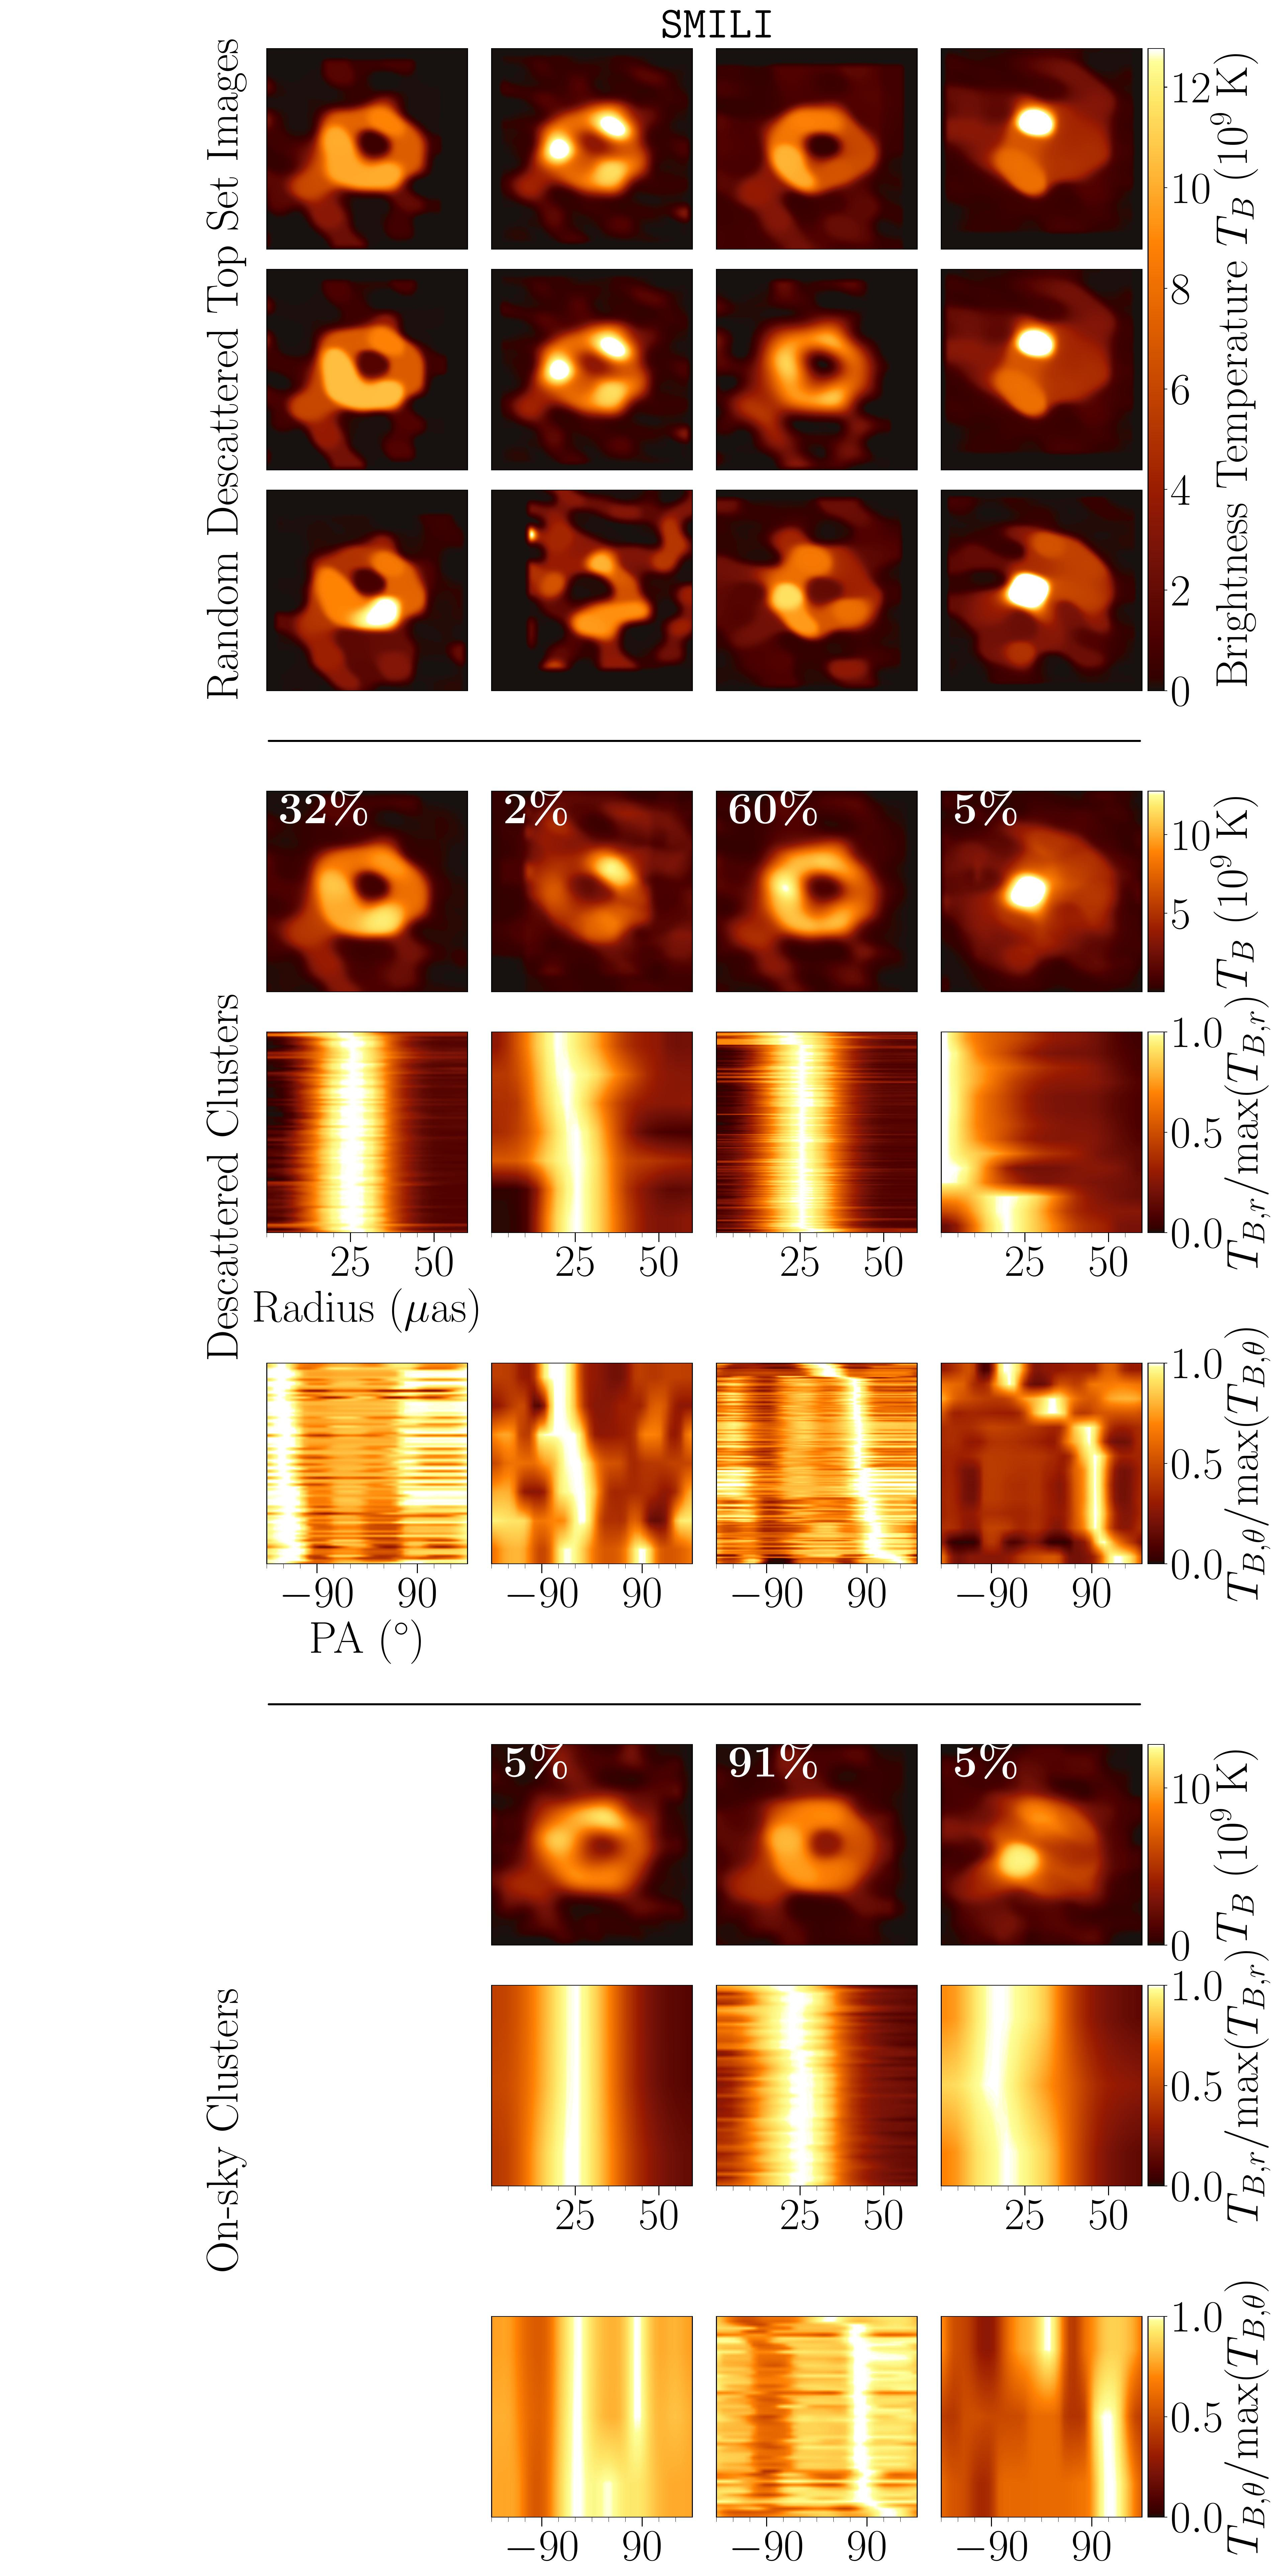}
    \caption{
    Classified summary of Sgr A* April 7 images with dynamical imaging pipelines of in \smili, where each movie is averaged over the observational time duration. 
    Top: averaged images of each cluster with symmetric (left), asymmetric (middle), and non-ring (right) structures.
    Middle: Radial distribution of of the intensity averaged to azimuthal direction among all images whose indices correspond to the vertical axis.
    Bottom: same as middle panel, but for the azimuthal distribution of brightness averaged to radial direction within $r_{\rm in}\leq r<r_{\rm max}$, where $(r_{\rm min}, r_{\rm max})=(20, 50)~ {\mu \rm as}$.
    }
    \label{fig:3class_allimages}
\end{figure}

As described in Section \label{sec::PreImaging_Considerations} the handling of the \magenta{intra-day} variation plays an essential role in exploring the structure of  \sgra.
In Section \ref{sec:sgra_images}, we introduced the variability noise model in the imaging parameter surveys and extracted the main image features mitigating the temporal variation effect. 
To crosscheck the independence of image characteristics on the specific assumption of the temporal variation, we perform the imaging survey introducing an alternative method for handling \magenta{intra-day} variability.
We adopt the dynamical imaging scheme to the full track observational data set without variability noise modeling.

We perform dynamical imaging parameter surveys with the same frame work of static ones, which is implemented in the imaging pipeline of \smili.
The dynamical imaging requires the time interval of the movie, and two \magenta{additional} imaging parameters (see \citep{johnson2017dynamical}). 
(Rt, Riの説明) 
We especially focus on the two scattering mitigation case: J18model1 and on-sky reconstructions and same parameter spaces of other imaging parameters.
Then we perform the 7 synthetic model parameter survey and extract the Top Sets with the same criteria of the static parameter surveys.

In Figure \ref{fig:4cls_dynamic}, we show the clustered results of all reconstructed Top Set images, where figure convention is the same as those of static imaging \magenta{results} in Section \ref{sec:sgra_images}.
Similar to static imaging survey, we can robustly separate all Top Set images into three ring and one non-ring clusters.
Both of the case of scattering mitigation, 
Figure ref shows that there are multimodal features in the all parameter surveys.
Existence of majority of ring and minority of non-ring.
Majority of position angle is different.

Parameter preference in Table .
Similar to static imaging, scattering mitigation helps us to increase the number of Top Set images.
$R_i$ indicates that the Sgr A* prefer the stable averaged images compared with low $R_i$ case.
$R_t$ has no preference.
In this way the conclusion does not change with different adoption of temporal variabilities.
