# Supplementary material for: First Sagittarius A* Event Horizon Telescope Results. III: Imaging of the Galactic Center Supermassive Black Hole
Source: arXiv:2311.09479 source file (2023-11-16)
Supplement: Supplementary file 2 [file appendix_synthetic.tex]

\section{Estimated gain uncertainty for synthetic data generation}

\begin{figure*}[t!]
\centering
\includegraphics[width=\linewidth]{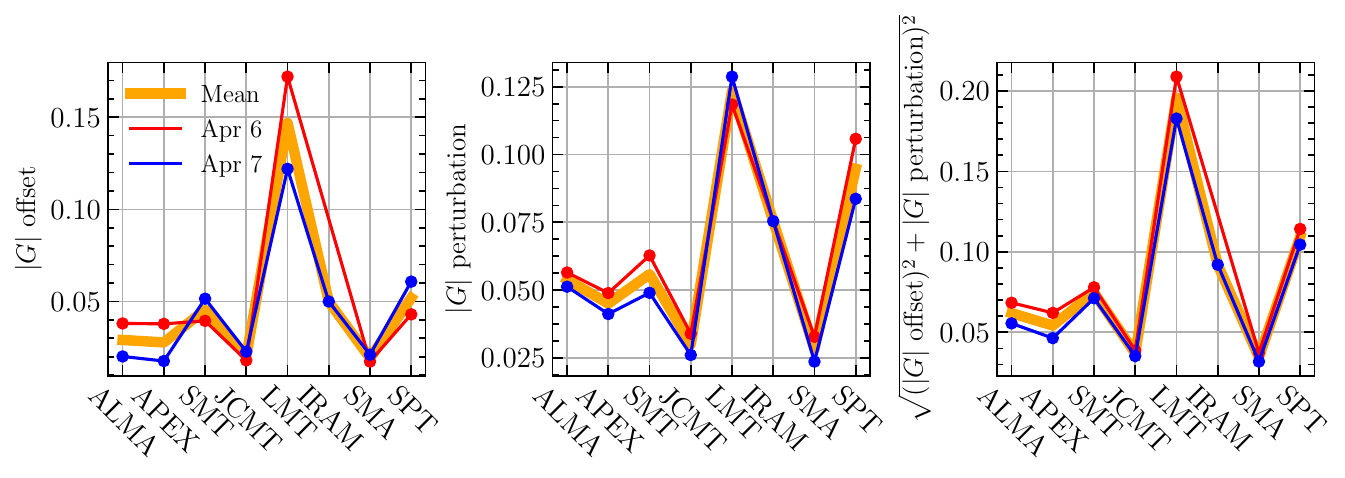}
\caption{}
\label{fig:synthetic_gain}
\end{figure*}

\begin{table}[h]
\caption{Estimated gain values from AGN imaging results.}
\centering
\begin{tabular}{c|cc|cc|cc}
\hline
 & \multicolumn{2}{c|}{Mean} & \multicolumn{2}{c|}{Apr 6} & \multicolumn{2}{c}{Apr 7} \\
\hline
Station & $g_{\rm offset}$ & $g_{\rm p}$ & $g_{\rm offset}$ & $g_{\rm p}$ & $g_{\rm offset}$ & $g_{\rm p}$\\
\hline
ALMA& 0.03& 0.05& 0.04& 0.06& 0.02& 0.05\\
APEX& 0.03& 0.05& 0.04& 0.05& 0.02& 0.04\\
SMT& 0.05& 0.06& 0.04& 0.06& 0.05& 0.05\\
JCMT& 0.02& 0.03& 0.02& 0.03& 0.02& 0.03\\
LMT& 0.15& 0.12& 0.17& 0.12& 0.12& 0.13\\
IRAM& 0.05& 0.08& ---& --- & 0.05& 0.08\\
SMA& 0.02& 0.03& 0.02& 0.03& 0.02& 0.02\\
SPT& 0.05& 0.09& 0.04& 0.11& 0.06& 0.08\\
\hline
\end{tabular}
\end{table}
